# Supplementary material for: From a Fourier-Domain Perspective on Adversarial Examples to a Wiener Filter Defense for Semantic Segmentation
Source: arXiv:2012.01558 source file (2021-04-21)
Supplement: Supplementary file 2 [file 08_Suppmentary_Material.tex]

\clearpage
\section{Supplementary Material}

\subsection{Additional Details on the Experimental Setup}
We provide detailed descriptions of the adversarial attacks we considered, the baseline defense methods used for comparison and the corresponding metrics used to report our results.
\subsubsection{Adversarial Attacks}
\label{subsec:Adversarial_Attacks}
According to Assion \textit{et al.}~\cite{Assion2019}, an adversarial attack consists of solving a constrained optimization problem with the constraint being the strength of the perturbation itself, usually in the form of an $L_{p}$ norm, mostly $L_{2}$ or $L_{\infty}$. Additionally depending on the attack input, an adversarial perturbation is usually computed in an iterative gradient based manner by repeated forward and backward passes through different layers of a CNN. An attack is said to be successful, if the optimization goal is reached within the permissible adversarial strength budget in a fixed number of iteration steps. These attacks are further classified depending on the optimization goal, adversary's knowledge, etc. For the sake of consistency, we follow attack conventions proposed by Assion \textit{et al.}~\cite{Assion2019}.  Additionally, we incorporated adversarial attacks from their framework \texttt{AidKit}\footnote{\url{https://aidkit.ai/}} for the scope of this work. The reason for this is mainly because, unlike existing frameworks such as \texttt{Foolbox}~\cite{rauber2017foolbox}, \texttt{Cleverhans}~\cite{papernot2018cleverhans} etc., which primarily work on the image classification task, \texttt{AidKit} employs attacks directly on the complex semantic segmentation task.

In this work, we consider \textit{two targeted} attacks, namely momentum FGSM (mFGSM)~\cite{Dong2018} and Metzen LLM~\cite{Metzen2017}, \textit{one untargeted} attack, namely Mopuri~\cite{Mopuri2018}, which at the same time is an image-agnostic attack and \textit{one confusion} based attack, namely iterative mirror (I.M.)~\cite{Metzen2017}. 
\begin{comment}
% Fig 1: Denoising qualitative example using WF
\begin{figure}[t!]
    \centering
    \includegraphics[width=\linewidth]{Figures/Denoising_example.pdf}
    \caption{\textbf{Visualization of Wiener filtering on clean data and perturbed/attacked data.} An example image $\boldsymbol{x} \in \mathcal{X}^{\text{val}}$ is cropped and visualized to demonstrate the effect of denoising using a Wiener filter $\boldsymbol{G}$ as shown in (\ref{eq:wiener_filter_h}) for the Mopuri attack~\cite{Mopuri2018} with $\epsilon=10$. Additionally, the MSE and the SSIM is reported with respect to the unfiltered clean data. It can be seen that Wiener filtering on clean data leads to an increase of MSE, but still keeps the SSIM at a reasonably high value. On the other hand, when being applied to perturbed/attacked data, the Wiener filtering successfully decreases the MSE, while at the same time it substantially increases the SSIM.}
    \label{fig:denoising_example}
\end{figure}{}
% Fig 1.2: Spatial v/s Frequency domain image

\makeatletter
\g@addto@macro\@maketitle{
  \begin{figure}[H]
  \setlength{\linewidth}{\textwidth}
  \setlength{\hsize}{\textwidth}
  \centering
  \includegraphics[height=3cm]{Figures/Spatial_vs_Frequency_Domain.pdf}
  \caption{\textbf{Image frequency spectra comparison} of clean v/s attacked image.}
  \label{fig:frequency_spectra_example}
  \end{figure}
}
\makeatother

\begin{figure*}[t!]
    \centering
    \includegraphics[width=\textwidth]{Figures/Spatial_vs_Frequency_Domain.pdf}
    \caption{\textbf{Image frequency spectra comparison} of clean v/s attacked image.}
    \label{fig:spatial_vs_frequency_domain}
\end{figure*}{}
\end{comment}
\paragraph{\textbf{Targeted attacks}}
%A targeted adversarial attack aims at fooling a CNN in a way, that the predicted pixel-wise probability scores $\boldsymbol{y}_{\kappa=\tau}(\boldsymbol{x})\in[0, 1]^{H\times W}$ for a given target class $\tau\in\mathcal{K}$ at any position does not match with the ground truth  $\hat{\boldsymbol{y}}_{\kappa=\tau}(\boldsymbol{x})\in\lbrace0, 1\rbrace^{H\times W}$ for an input image $\boldsymbol{x}$ having width $W$ and height $H$. We elaborate on the two targeted attacks used in this work as follows.
A targeted adversarial attack aims at fooling a CNN in a way, that the predicted pixel-wise probability scores $\boldsymbol{y}_{\tau}=\mathfrak{F}_{\tau}(\boldsymbol{x}, \boldsymbol{\theta})\in[0, 1]^{H\times W\times 1}$ for a given target class $\tau\in\mathcal{S}$ and input image $\boldsymbol{x}\in\mathbb{G}^{H\times W\times C}$ are zero.
Note that $\boldsymbol{y}_{\tau}$ can be considered as a subtensor of the complete network output $\boldsymbol{y}$ containing probability scores for all classes $s\in\mathcal{S}$.
We elaborate on the two targeted attacks used in this work as follows.

\textbf{Momentum FGSM:} Goodfellow \textit{et al.}~\cite{Goodfellow2015} originally proposed the fast gradient sign method (FGSM) which was later on extended to iterative FGSM by Kurakin \textit{et al.}~\cite{Kurakin2017a}. Dong \textit{et al.}~\cite{Dong2018} further boosted the iterative FGSM by integrating a momentum term into the iterative process, resulting in a much stronger and stable attack called momentum FGSM (mFGSM). To find adversarial examples $\boldsymbol{x}^{\text{adv}}$ within the $\epsilon$ vicinity under the $L_\infty$ norm of a real example $\boldsymbol{x}$, the mFGSM attack can be computed by 
\begin{equation}
    \boldsymbol{x}^{\text{adv}}_{t+1} = \boldsymbol{x}^{\text{adv}}_{t} - \alpha \cdot \text{sign}(\boldsymbol{g}_{t+1}),
    \label{eq:adv_x_t+1}
\end{equation}
where $\alpha=\epsilon/T$ denotes the step size, $t\in [1,2,\dots,T]$ denotes the iteration step, $\text{sign}(\cdot) \in \{\pm 1\}^{H \times W \times C}$  denotes the sign function and
\begin{equation}
    \boldsymbol{g}_{t+1} = \mu \cdot \boldsymbol{g}_{t} + \frac{J(\boldsymbol{x}^{\text{adv}}_{t}, \boldsymbol{y}_{\tau})}{||\nabla_{\boldsymbol{x}}J(\boldsymbol{x}^{\text{adv}}_{t}, \boldsymbol{y}_{\tau})||_{1}}.
    \label{eq:mfgsm_gradient}
\end{equation}
denotes the accumulated gradient.
%Note that $\mu$ here denotes the momentum constant. The objective of the attack is to minimize the output probability score vector $\boldsymbol{y}_{\tau} = P(\kappa=\tau|\boldsymbol{x})$ with $\tau$ being the target class that the adversary wants to erase (e.g. pedestrian). This is done by solving the following constrained optimization problem
Note that $\mu$ here denotes the momentum constant.
The objective of the attack is to minimize the output probability scores $\boldsymbol{y}_{\tau}$ for a particular target class $\tau$, e.g., pedestrians, leading to the constrained optimization problem
\begin{equation}
     \underset{\boldsymbol{r}}{\rm{min}}\hspace{2pt} J(\boldsymbol{x}^{\text{adv}}, \boldsymbol{y}_{\tau}) \hspace{5pt} \textit{\rm{s.t.}} \hspace{5pt} ||\boldsymbol{r}||_{p} \leq \epsilon,
\end{equation}
where the loss $J(\cdot)$ is defined as 
\begin{equation}
    J(\boldsymbol{x}^{\text{adv}}, \boldsymbol{y}_{\tau}) = ||\boldsymbol{y}_{\tau}(\boldsymbol{x} + \boldsymbol{r})||_{2}.
\end{equation}
For simplicity we left out the subscript $t$.
Note that Dong \textit{et al.}~\cite{Dong2018} proposed to use the cross-entropy loss instead of the $L_{2}$ loss.
Nonetheless, using the $L_{2}$ loss lead to stronger attacks in semantic segmentation. We did not investigate this observation further.

\textbf{Metzen LLM:} Metzen \textit{et al.}~\cite{Metzen2017} showed the existence of targeted, universal adversarial attacks for state-of-the-art semantic segmentation neural networks. Considering a set of images $\mathcal{X}$, Metzen \textit{et al.} proposed to solve
\begin{equation}
    \underset{\boldsymbol{r}}{\rm{min}}\hspace{2pt} \mathbb{E}_{\boldsymbol{x} \in \mathcal{X}} [J^{\text{CE}}(\boldsymbol{y}(\boldsymbol{x} + \boldsymbol{r}), \boldsymbol{m}^{\text{target}}(\boldsymbol{x}))] \hspace{5pt} \textit{\rm{s.t.}} \hspace{5pt} ||\boldsymbol{r}||_{p} \leq \epsilon,
    \label{eq:metzen}
\end{equation}
where $J^{\text{CE}}$ denotes the cross-entropy loss and $\boldsymbol{m}^{\text{target}}(\boldsymbol{x})\in\mathcal{S}_{\tau}^{H\times W}$, with $\mathcal{S}_{\tau}=\mathcal{S}\setminus\lbrace \tau\rbrace$, denotes a fake segmentation mask.
The fake segmentation mask is created beforehand by replacing a certain target class $\tau$ in the original network prediction of $\boldsymbol{x}$ by its nearest neighbor class following a 2D minimum Euclidean distance calculation.
We refer the interested reader to \cite{Metzen2017} for detailed formulations of $\boldsymbol{m}^{\text{target}}$.
The optimization problem is solved in an iterative manner similar to (\ref{eq:adv_x_t+1}), with the difference of the gradient $\boldsymbol{g}_{t+1}$ being
\begin{equation}
    \boldsymbol{g}_{t+1} = \nabla_{\boldsymbol{x}} J^{\text{CE}}(\boldsymbol{y}(\boldsymbol{x}_{t} + \boldsymbol{r}_{t}), \boldsymbol{m}^{\text{target}}(\boldsymbol{x}_{t})).
    \label{eq:metzen_gradient}
\end{equation}
Technically, given such an attack formulation, an attacker can simply create any number of fake segmentation masks by manually designing $\boldsymbol{m}^{\text{target}}(\boldsymbol{x})$ beforehand following any reasonable design rule. We show an example how this could be done in the iterative mirror attack next.
\paragraph{\textbf{Confusion-based attacks}} 
Although some attackers might target specific classes, adversarial attacks can also be created with an aim of causing confusion in the output. One example of such an attack is presented by Assion \textit{et al.}~\cite{Assion2019} in their framework \texttt{AidKit}, namely iterative mirror.
% Fig 5.2: Epsilon and Iteration Variation
\begin{figure*}[t!]
    \centering
    \includegraphics[width=17cm]{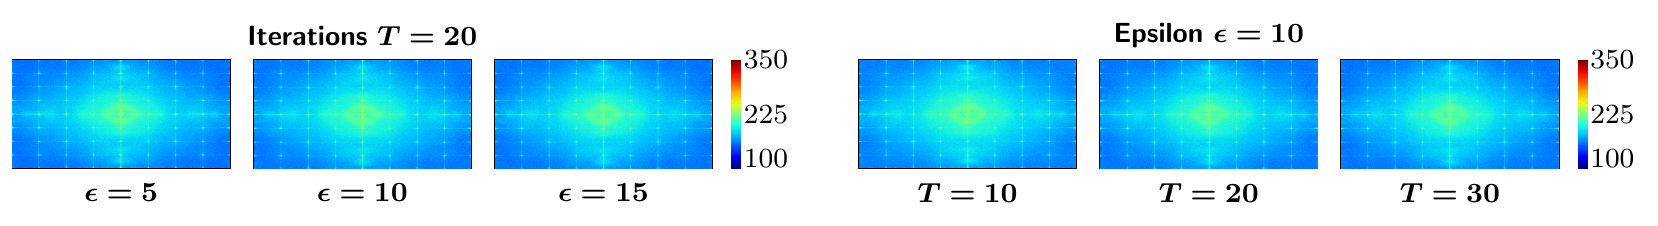}
    \caption{\textbf{Visualization of average amplitude spectra of adversarial perturbations} varied along attack parameters: \textbf{attack strength $\epsilon$,} and \textbf{total number of iterations $T$.}}
    \label{fig:epsilon_and_iteration_variation}
\end{figure*}
% Fig 5.3: Mopuri Layer Variation - ICNet Figure
\begin{figure*}[t]
    \centering
    \includegraphics[width=17cm]{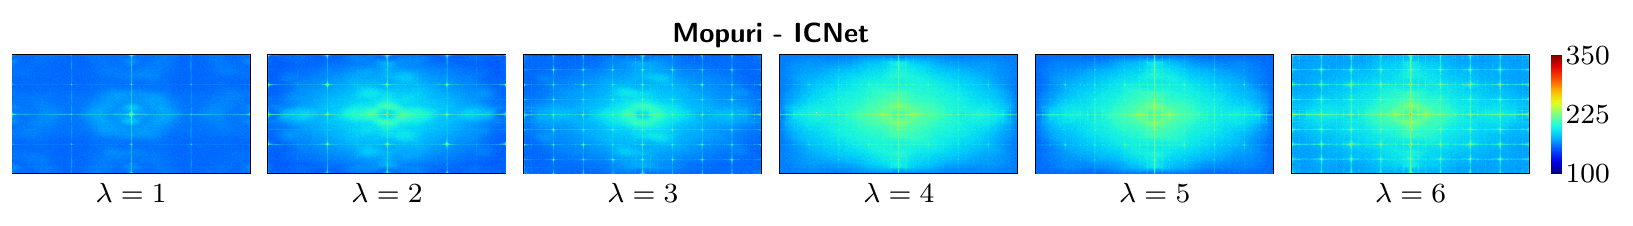}
    \caption{\textbf{Visualization of average amplitude spectra of adversarial perturbations} computed for the Mopuri attack on the ICNet model varied along attacked convolutional layer $\lambda$. We estimate $\mathbb{E}[|\mathcal{F}(\boldsymbol{x}^{\text{adv}} - \boldsymbol{x})|]$ for $100$ randomly chosen training set images.}
    \label{fig:mopuri_layer_variation}
\end{figure*}
% Fig 5.4: Mopuri Layer Variation - FCN Figure
\begin{figure*}[t]
    \centering
    \includegraphics[width=15cm]{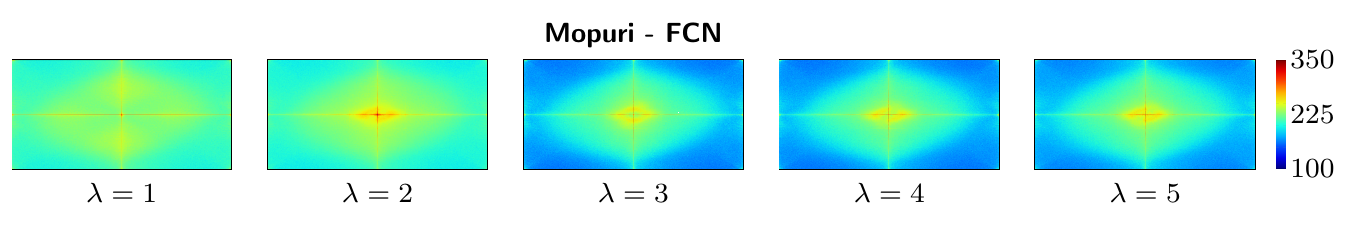}
    \caption{\textbf{Visualization of average amplitude spectra of adversarial perturbations} computed for the Mopuri attack on the FCN model varied along attacked convolutional layer $\lambda$. We estimate $\mathbb{E}[|\mathcal{F}(\boldsymbol{x}^{\text{adv}} - \boldsymbol{x})|]$ for $100$ randomly chosen training set images.}
    \label{fig:mopuri_layer_variation_FCN}
\end{figure*}

\textbf{Iterative mirror:} Inspired by the Metzen \textit{et al.} attack, Assion \textit{et al.} proposed an alternative formulation of the target fake segmentation map $\boldsymbol{m}^{\text{target}}$.
We now consider $h$ and $w$ as the vertical and horizontal position within any segmentation map $\boldsymbol{m}\in\mathcal{S}^{H\times W}$, respectively.
By simply following the rule
\begin{equation}
    m^{\text{target}}_{h,w} = m_{h,W-w},
\end{equation}
we can perform a mapping of the pixels on the right to pixels on the left and vice versa.
In a sense, the resulting $\boldsymbol{m}^{\text{target}}$ can be considered as the mirrored image of $\boldsymbol{m}$.
In our experiments we mirrored the original predicted segmentation of $\boldsymbol{x}$.
The rest of the optimization method is the same as shown in (\ref{eq:adv_x_t+1}), (\ref{eq:metzen}) and (\ref{eq:metzen_gradient}) which leads to a mirrored segmentation output.

\paragraph{Untargeted attacks}
An untargeted attack does not have a specific preference in a particular class of the output, but rather aims at as many misclassifications as possible.

\textbf{Data-Free Mopuri:} Mopuri \textit{et al.}~\cite{Mopuri2018} proposed a universal adversarial attack that is image- and task-agnostic and generalizes across several architectures. The key idea is to optimize the attack such that the computed perturbation maximizes feature map activations $\boldsymbol{f}_{\lambda}(\cdot)$ of a subset of layers $\mathcal{L}$, with $\lambda \in \mathcal{L}$, thereby implying a lot of misclassifications. This is achieved by solving the following optimization problem
\begin{equation}
    \underset{\boldsymbol{r}}{\rm{min}}\Big(-\rm{\log}(\prod_{\lambda \in \mathcal{L}}^{}||\boldsymbol{f}_{\lambda}(\boldsymbol{r}_{0} + \boldsymbol{r})||_{2})\Big) \hspace{5pt} \textit{\rm{s.t.}} \hspace{5pt} ||\boldsymbol{r}||_{\textit{p}} \leq \epsilon,
    \label{eq:mopuri}
\end{equation}
where $\boldsymbol{f}_{\lambda}(\cdot)$ denotes the feature map activations of a layer $\lambda \in \mathcal{L}$ and $\boldsymbol{r}_{0}$ is a randomly initialized perturbation at $t=0$. The optimization problem is solved in an iterative manor.
For the exact iterative update rule, we refer the interested reader to \cite{Mopuri2018}.
Note that the optimization objective does not need any input clean images, hence the algorithm itself is already \textit{image-agnostic}. This attack also does not need to know anything about the output of the neural network, making it also a \textit{task-agnostic} attack.

\subsubsection{Baseline Defense Methods}
For the complex semantic segmentation task, we limit our investigations to adversarial defenses of type \textit{input transformation}, specifically the ones that do not need additional retraining. This is done to avoid additional computational overhead. We investigate two well-known categories of such defenses, namely image compression~\cite{Dziugaite2016} and feature squeezing~\cite{Xu2017} methods. We present details of both these methods next.

\paragraph{\textbf{Image Compression}}  Image compression is a well known technique of reducing redundancy in an image in an efficient form. As an adversarial defense, JPEG compression and JPEG 2000 compression are well-known.

\textbf{JPEG compression} was first proposed by Dzuigaite \textit{et al.}~\cite{Dziugaite2016} and further investigated in ~\cite{Aydemir2018, Shaham2018, Prakash2018}. JPEG compression is mainly a lossy compression method that first transforms an image into $8\times 8$ blocks and converts them to frequencies using the discrete cosine transform (DCT). Next, in order to reduce redundancy, it suppresses high frequencies using quantization, thereby introducing unwanted blocking artifacts, specifically at high compression rates. 

\textbf{JPEG 2000 compression} was proposed by Aydemir \textit{et al.}~\cite{Aydemir2018} in order to alleviate the shortcomings of JPEG compression. As JPEG 2000 uses wavelet transforms over DCT, and does not need image transformation into blocks, blocking artifacts are thereby not introduced, even at high compression rates. However, Aydemir \textit{et al.} concluded that a good quality or lossless compression does not necessarily mean a good defense, as it also tends to unknowingly preserve the adversarial perturbations.

\paragraph{\textbf{Feature Squeezing}} Xu \textit{et al.}~\cite{Xu2017} introduced feature squeezing as a bunch of techniques that aim at reducing the input space features, thereby reducing the available search space for an adversary. Although there are many such methods possible, they explored bit-depth reduction and median blurring and non-local means smoothing techniques. These methods are, however, proposed from an adversarial detector perspective.

\textbf{Median Blurring (MB)}~\cite{Aydemir2018} is a type of local \textit{spatial smoothing} method widely known in image processing to reduce noise. A median filter is applied locally where each pixel is replaced with the median of a few of its neighboring pixels. Similarly, one can also perform mean or Gaussian smoothing.

\textbf{Non-Local Smoothing (NLM):} In contrast, \textit{non-local smoothing} algorithm utilizes much larger areas of the image for smoothing instead of just neighboring pixels. More specifically, in NLM~\cite{Buades2005}, every pixel is replaced by a weighted average of all other pixels in the image where the weightage is computed based on how similar each pixel is to the target pixel.

\textbf{Bit-Depth Reduction:} An 8-bit grayscale image corresponds to  $2^{8} = 256$ available colors. In contrast, an 8-bit RGB image corresponds to 24 bits per pixel (8 bits per channel), and therefore $2^{24} \approx 16$ million colors. While most humans can recognize black and white images just as good as color images, it is often hypothesized that reducing the number of available color bits might not harm the classification performance as such and thereby also reduce the search space for an adversary.
%Fig: Upsampling example
\begin{figure*}[t!]
    \centering
    \includegraphics[width=\linewidth]{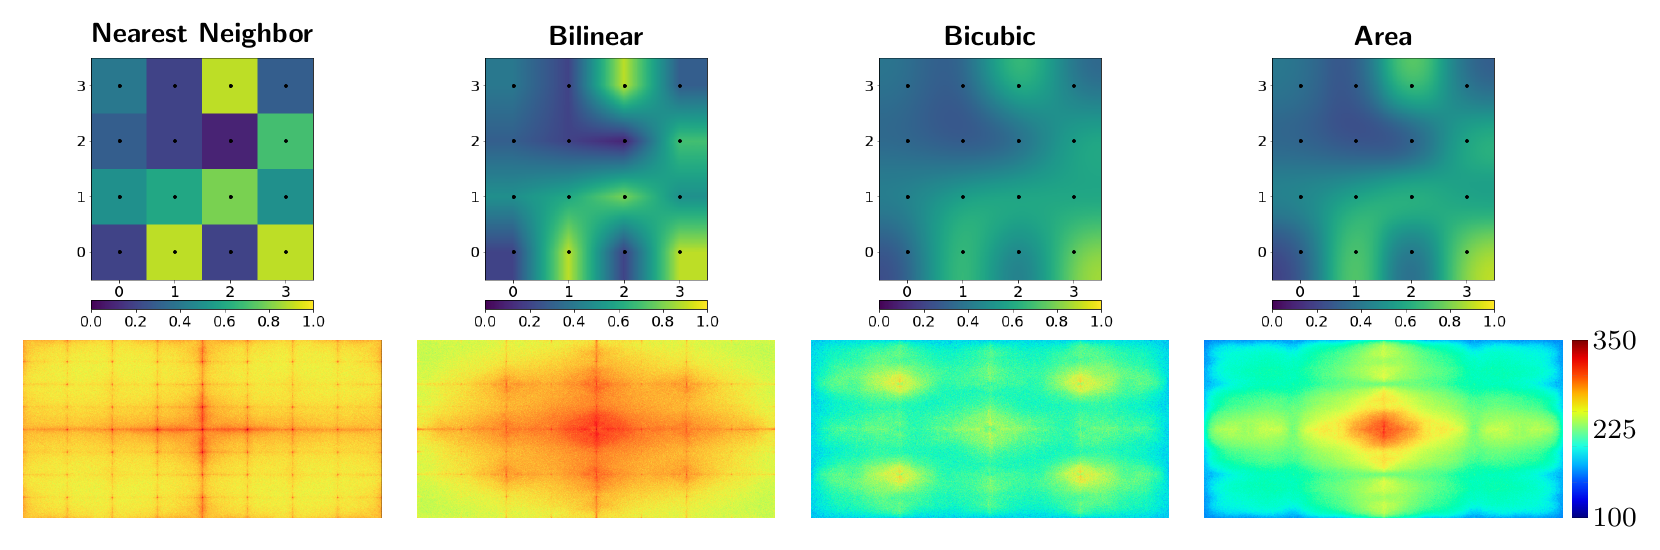}
    \caption{\textbf{Different upsampling methods} in the ICNet~\cite{Zhao2018a} architecture lead to different types of artifacts in the resulting adversarial perturbations. For each method, we visualize in the upper row the interpolation of $[0,3] \times [0,3]$ consisting of 16 unit square points patched together. Color indicates function value. The black dots are the locations of the prescribed data being interpolated. \textbf{
    Nearest neighbor interpolation} tends to output pixelated images due to sudden variations in neighboring pixels. This effect is reduced by incorporating more advanced interpolation methods such as \textbf{bilinear interpolation} and \textbf{bicubic interpolation}, however at a higher computation cost. \textbf{Area interpolation} is also known as \textbf{adaptive average pooling} is a high quality interpolation method that ensures anti-aliasing using a low-pass averaging filter (LPF). For each method in the lower row, we visualize $|\mathcal{F}(\boldsymbol{r})|$ computed on a single fixed image from the Cityscapes data set, keeping constant attack parameters.}
    \label{fig:upsamplers}
\end{figure*}{}
% Fig 1: ICNet Architecture
\begin{figure}[t!]
    \centering
    \includegraphics[width=\linewidth]{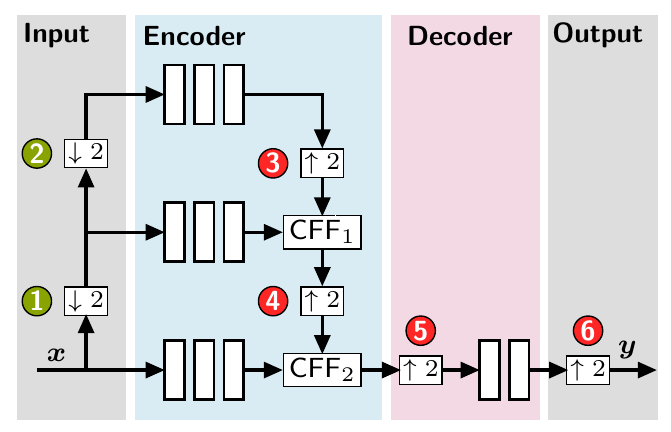}    \caption{\textbf{Simplified ICNet~\cite{Zhao2018a}} architecture overview. The input of the ICNet is an RGB image processed at three different resolutions. The encoder processes each of the three (downsampled) inputs separately, following a cascade feature fusion (CFF) at the end. Finally, the decoder performs upsampling to obtain a full-resolution semantic segmentation map at the output. Please note that the \textbf{default interpolation method} used in the ICNet is \textbf{bilinear interpolation}.}
    \label{fig:ICNet}
\end{figure}
\subsubsection{Evaluation Metrics}
Our results are reported on the following metrics:

\paragraph{Mean Squared Error (MSE)}
We compute the mean squared error between the attacked image $\boldsymbol{x}^{\text{adv}}$ and the attacked denoised image $\hat{\boldsymbol{x}}$ by
\begin{equation}
    MSE(\boldsymbol{x}^{\text{adv}},\hat{\boldsymbol{x}}) = \frac{1}{HWC}\sum_{h=0}^{H-1}\sum_{w=0}^{W-1}\sum_{c=0}^{C-1} (x_{h,w,c}^{\text{adv}} - \hat{x}_{h,w,c})^{2},
\end{equation}
where $h,w,c$ denote the indices of the images along height, width and channels, respectively. Additionally, we also compute the MSE between the clean image $\boldsymbol{x}$ as well as its clean filtered image $\boldsymbol{x}'$. This is computed by $\boldsymbol{x}'=g(\boldsymbol{x})$, where $g(\cdot)$ is the denoising method.
\paragraph{Structural Similarity Metric (SSIM)}
We also compute the structural similarity index metric (SSIM) according to~\cite{Wang2004} on the attacked image $\boldsymbol{x}^{\text{adv}}$ and the attacked denoised image $\hat{\boldsymbol{x}}$ as follows
\begin{equation}
    SSIM(\boldsymbol{x}^{\text{adv}},\hat{\boldsymbol{x}}) = [\phi(\boldsymbol{x}^{\text{adv}},\hat{\boldsymbol{x}})]^{\alpha} \cdot [\chi(\boldsymbol{x}^{\text{adv}},\hat{\boldsymbol{x}})]^{\beta} \cdot [\psi(\boldsymbol{x}^{\text{adv}},\hat{\boldsymbol{x}})]^{\gamma},
\end{equation}
where $\phi(\cdot,\cdot)$, $\chi(\cdot,\cdot)$, $\psi(\cdot,\cdot)$ are mathematical functions denoting a measure of luminosity, contrast, and saturation, respectively, and $\alpha, \beta, \gamma$ are constants. We refer the reader to~\cite{Wang2004} for detailed definitions of these functions. The SSIM values range from 0 (lowest) to 1 (highest). Similarly we also report results on SSIM between the clean image $\boldsymbol{x}$ and the clean filtered image $\boldsymbol{x}'$.

\paragraph{Mean Intersection over Union (mIoU)}:
For semantic segmentation, \textit{mean intersection-over-union} (mIoU) is commonly used to evaluate the performance of the network. It is computed by
\begin{equation}
    mIoU = \frac{1}{|\mathcal{S}|}\sum_{s\in\mathcal{S}}^{}\frac{TP(s)}{TP(s) + FP(s) + FN(\kappa)},
\end{equation}
where $TP(s)$, $FP(s)$, $FN(s)$ indicate class specific true positives, false positives, and false negatives, respectively.

\subsection{Additional Results}

\subsubsection{Fourier Domain Analysis}
In Fig.~\ref{fig:epsilon_and_iteration_variation}, we demonstrate results of our ablation study on the effect of varying attack parameters, namely epsilon $\epsilon$ and number of iterations $T$. These results are reported for the attack on the ICNet model using an $L_\infty$ norm. The results of this experiment indicate that varying attack parameters tend to have similar patterns, indicating similar SNRs.

\textbf{Effect of varying layers in the Mopuri attack.} In the attack generation process, unlike the mFGSM, Metzen, and I.M. attacks, which need gradients to be processed through the entire network architecture, the Mopuri attack, by design, needs access to gradients from a subset of layers in the network starting from the first layer up to layer $\lambda$. The layers deeper than $\lambda$ till the very end of the network are not considered for the gradient computation. We investigate the effect of varying convolution layers $\lambda$ for the Mopuri attack and visualize the average amplitude spectra in Fig.~\ref{fig:mopuri_layer_variation}. Surprisingly this time, \textit{we observed clear variations in the grid-shaped artifacts by varying the underlying layers.} This finding further reaffirms our earlier hypothesis on the connection of the network architecture and its corresponding artifacts. Interestingly, the artifacts of Mopuri (attacked on the last convolutional layer \texttt{conv6}) are similar to artifacts emerging from the other attack types. This is mainly because, in this case, for all attacks, the number of layers used for gradient computation remains the same.
\begin{comment}
These observations lead us to an important finding, i.e., the information processing through different layers of a CNN might lead to different artifacts that are observable in the frequency domain. From a signal processing perspective, the signal (in this case images) are passed through several downsampling and upsampling layers commonly found in CNNs which might lead to several artifacts in the frequency domain. Since, these perturbations are usually always computed through some network type, a research towards finding which architecture leads to which specific patterns might help us in defending against many kinds of unseen attacks in the future. 
\end{comment}

Next, in Fig.~\ref{fig:mopuri_layer_variation_FCN}, we show the results of varying convolutional layers $\lambda$ in the Mopuri attack computed on the FCN model, instead of ICNet (as shown in Fig. 4 in the paper). In comparison to earlier results on ICNet, different layers tend to have little effect on the underlying artifacts. These results are somewhat expected, considering different layers in the FCN are predominantly similar, in the way information is processed, unlike in the ICNet. We leave a detailed study of the effect of individual layer types (found commonly in CNNs) on the resulting artifacts to future study.

\textbf{Source of artifacts:} Inspired by Odena et al.~\cite{Odena2016} and Wang et al.~\cite{Wang2020_3}, we hypothesize that \textit{the observed grid-shaped artifacts in the ICNet architecture are caused by the underlying upsampling/downsampling layers}. In order to verify this hypothesis, we perform an experiment to investigate the effect of different upsampling methods.

However, first we take a deeper look into the ICNet architecture~\cite{Zhang2018a} as shown in Fig.~\ref{fig:ICNet}. From this figure, we can see that the input image $\boldsymbol{x}$ is first downsampled two times to $1/2$ and $1/4$ of the original resolution using bilinear interpolation (steps 1 and 2). Thereafter, these three resolution inputs are fed through three parallel layers in the encoder part of the network, each consisting of different sets of stacked convolution layers.  The outputs of these three layers are fused together using two fusion layers ($\text{CFF}_1$ and $\text{CFF}_2$) called cascade feature fusion (CFF). Prior to each CFF step, a bilinear upsampling is performed to ensure resolution compatibility (steps 3 and 4). Finally, the output of the encoder (after $\text{CFF}_2$) is then passed to the decoder which again consists of two bilinear upsampling layers (steps 5 and 6) separated by two convolution layers in between. Step 6 finally produces the desired full-resolution semantic segmentation map. From the architecture, one can see that there exist six places (downsampling/upsampling steps 1-6), where bilinear interpolation is performed.

In order to support our hypothesis, we now change each of the default \textit{bilinear interpolation} steps (steps 1-6) to three different types: a) \textit{nearest neighbor}, b) \textit{bicubic interpolation} and c) \textit{area interpolation}, also known as \textit{adaptive average pooling}. In each case, we recompute the attack, keeping all attack parameters constant (mFGSM attack with $\epsilon=10$ and $T=20$). As seen from the results in Fig.~\ref{fig:upsamplers}, we make three important observations. First, \textit{the type of artifacts observed were clearly different for each interpolation method}. Second, the \textit{nearest neighbor method} exhibits an even stronger grid than the default \textit{bilinear upsampling} method. Third, the \textit{bicubic interpolation} method and \textit{area interpolation}, being more advanced upsampling methods than the other two, have strikingly different patterns. These observations are in line with our hypothesis that \textit{the type of interpolation method used has a strong effect on the underlying artifacts observed}.

Finally, we investigated which of the six interpolation steps (steps 1-6) has the strongest effect on the resulting artifacts, using an in-depth ablation study. Our results showed that \textit{input steps 1 and step 2 have the strongest effect on the resulting artifacts. }

We now provide a possible explanation for this finding. Please note that, as seen from the architecture in Fig.~\ref{fig:ICNet}, the input steps 1 and 2 (unlike steps 3-6) are downsamplers in the forward pass. However, during the backward pass for gradient computation, the roles get reversed, i.e., steps 1 and 2 are computed as upsamplers. Since in an adversarial attack, the gradient is computed w.r.t. the input image $\boldsymbol{x}$, steps 1 and 2 are now the output steps of the attack. Given such a setup, the final two steps of the attack (steps 1 and 2) are two strong consecutive upsamplers, which is likely to leave stronger artifacts in the output. One might expect, that if we apply a smoothing filter at the attack output, we might expect the effect of the artifacts to be reduced. We leave out a detailed study of types of interpolation methods and their effect on DNNs as scope of future work.

\subsubsection{Wiener filters as an Adversarial Defense}
We provide detailed results on the effectiveness of using Wiener filters as an adversarial defense. Please note that the results shown in Fig. 5 a) and 5 c) of the paper are adapted/summarized in Tab.~\ref{tab:wiener_mse_ssim_results}, ~\ref{tab:wiener_mIoU_results_ICNet} and ~\ref{tab:wiener_mIoU_results_FCN}.

\paragraph{SSIM and MSE Results}
The effect of the Wiener filter based denoising in comparison to existing methods on traditional metrics such as MSE and SSIM are reported in Tab.~\ref{Table:ssim_mse_results}. In the paper, we only reported the final aggregated summary, however, detailed results are presented here. Additionally, different combinations ($\epsilon$ and attack mismatch between creation and evaluation of Wiener filter) of Wiener filters are also reported here. More specifically, we denote the following variations of Wiener filters:
\begin{enumerate}
    \item $\boldsymbol{G}^{(\text{Metzen})}$ - a single attack Wiener filter~(as in Eq. \ref{eq:wiener_filter_single_attack}) trained on Metzen~\cite{Metzen2017} attack.
    \item $\boldsymbol{G}^{(\text{mFGSM})}$ - a single attack Wiener filter~(as in Eq. \ref{eq:wiener_filter_single_attack}) trained on mFGSM~\cite{Dong2018} attack.
    \item $\boldsymbol{G}^{(\text{a})}$ - attack matched setting where the type of attack used for training the WF is the same as the type of attack used in evaluation.
\end{enumerate}
Essentially, more or less each combination of Wiener filter that we tried excelled all the remaining state of the art denoising methods on both SSIM as well as MSE. The results show significant improvement after denoising on both attacked images (see column Attacked Denoised) and on clean images (see column Clean Filtered).

\paragraph{mIoU Results}
The results of Fig. 5 (c) in the paper are adapted from the right-most column of Tab.~\ref{tab:mIoU_results_ICNet} and Tab.~\ref{tab:mIoU_results_FCN}. Additionally, as before, we present additional results of different variants of Wiener filters with an $\epsilon$ and attack mismatch. From these results, we can conclude that Wiener filters tend to work well under various mismatched conditions, which is better than other methods. The reason for their success can be attributed directly to their frequency-based denoising nature since the artifacts they try to suppress remain more or less the same (see Fig.~\ref{fig:epsilon_and_iteration_variation}) even under various mismatched conditions.

% Tab 5.1: SSIM and MSE Results 
% Table for MSE and SSIM on the validation set
\begin{table*}[t!]
\centering
\caption{\textbf{Comparison of SSIM and MSE metrics} with and without denoising for the ICNet~\cite{Zhao2018a} model trained on the Cityscapes dataset. We report averaged SSIM and MSE performance over the entire \textbf{validation set} images w.r.t. the reference clean images $\boldsymbol{x}$ of (a) the \textbf{attacked} images $\boldsymbol{x}^{\text{adv}}$ \textbf{across all attacks} with strength $\epsilon=10$ based on the $\boldsymbol{L_{\infty}}$ \textbf{norm}, (b) the corresponding \textbf{attacked denoised} images $\hat{\boldsymbol{x}}$, and (c) the \textbf{clean filtered} images $\boldsymbol{x}'$. In the case of Wiener filtering, the filters are computed over clean and adversarial images with strength $\epsilon=5$ (\textbf{unmatched} conditions) and $\epsilon=10$ (\textbf{matched} conditions) spanning the entire training set.  An increase in SSIM after denoising, and a corresponding decrease in MSE are desired. The best denoised results are marked in \textbf{bold}, second best \underline{underlined}, with the Wiener filter upper limit and single-attack Wiener filters $\boldsymbol{G}^{(a)}$, $\boldsymbol{G}^{(\text{Metzen})}$, $\boldsymbol{G}^{(\text{mFGSM})}$ being excluded. The values in Fig. 5(a) of the paper are taken from the \textbf{Attacked Denoised} column of this table.}
\label{Table:ssim_mse_results}
\resizebox{0.8\linewidth}{!}{

\begin{tabular}{l|ll|c|cc|c|cc} 
\toprule

 \multicolumn{3}{c|}{}   & \multicolumn{3}{c|}{\textbf{Average SSIM}} & \multicolumn{3}{c}{\textbf{Average MSE}} \\ \cline{4-9}
                                
                                     \multicolumn{3}{c|}{\textbf{Defense Method}}                  & \multicolumn{1}{c}{\multirow{2}{*}{\textbf{Attacked}}} & \textbf{Attacked} & \textbf{Clean} & \multicolumn{1}{c}{\multirow{2}{*}{\textbf{Attacked}}} & \textbf{Attacked} & \textbf{Clean} 
                                \\
                                   \multicolumn{3}{c|}{}                      & \multicolumn{1}{c}{} &  \textbf{Denoised}& \textbf{Filtered} & \multicolumn{1}{c}{} &  \textbf{Denoised} & \textbf{Filtered} 
                                \\ \hline
 \multirow{9}{*}{\rotatebox{90}{Wiener Filter WF (Ours)}} & $\boldsymbol{G}$ (upper limit) & & \multirow{14}{*}{$0.89$} & $0.95$ & $1.00$ & \multirow{14}{*}{$78.76$} & $47.80$ & $0.00$  \\  

\cline{2-3} \cline{5-6} \cline{8-9}
      & \multirow{2}{*}{$\boldsymbol{G}^{(a)}$}  & matched   &  &  $\boldsymbol{0.95}$ & $0.99$ &  & $57.20$ & $14.07$  \\ %\cline{3-9} 
    
       &  & unmatched   &   & $0.93$ & $1.00$ & & $\underline{56.04}$ & $5.12$ \\
   \cline{2-3} \cline{5-6} \cline{8-9}
    
     %\cline{3-9} 

       & \multirow{2}{*}{$\boldsymbol{G}^{(\text{Metzen})}$}  & matched &   & $0.92$ & $1.00$& & $59.11$  & $4.38$ \\ %\cline{3-9} 
    
       &  & unmatched  &   & $0.91$  & $1.00$  & & $62.54$ & $2.23$ \\
    \cline{2-3} \cline{5-6} \cline{8-9}
       & \multirow{2}{*}{$\boldsymbol{G}^{(\text{mFGSM})}$}  & matched & & $\underline{0.94}$ & $0.98$ & & $65.96$  & $23.99$ \\ %\cline{3-9} 
    
       &  & unmatched  &  & $0.93$  & $0.99$ & & $58.19$  & $8.47$ \\
    \cline{2-3} \cline{5-6} \cline{8-9}
    
       & \multirow{2}{*}{$\boldsymbol{G}^{(\mathcal{A})}$}  & matched &    & $\underline{0.94}$ & $0.99$& & $59.18$ & $11.38$\\
     
          &  & unmatched  &   & $0.92$  & $1.00$ & & $59.25$  & $4.28$ \\
    
    \cline{1-3} \cline{5-6} \cline{8-9}
                                                  \multicolumn{3}{c|}{JPEG compression} &   & $0.90$ & $0.98$ & & $82.50$  & $13.92$ \\
                         %\cline{3-9}
                                            \multicolumn{3}{c|}{JPEG 2000 compression}    &   & $0.89$ & $1.00$ & & $80.42$  & $0.00$ \\
                                                                     \multicolumn{3}{c|}{NL Means}     &   & $0.92$ & $0.98$ & & $60.71$  & $8.61$ \\
                                                        \multicolumn{3}{c|}{Median Blur}     &  & $0.90$  & $0.98$  & & $84.20$   & $16.17$  \\
            
             \multicolumn{3}{c|}{Bit Depth Reduction} &  & $0.86$  & $0.95$  & & $86.87$   & $17.48$ \\\cline{1-3} \cline{5-6} \cline{8-9}
                               \multicolumn{3}{c|}{WF $\boldsymbol{G}^{(\mathcal{A})}$ (matched) + NL Means}     &   & $\underline{0.94}$ & $0.97$ & & $57.03$  & $23.74$ \\
                                   \multicolumn{3}{c|}{WF $\boldsymbol{G}^{(\mathcal{A})}$ (unmatched) + NL Means}     &   & $\underline{0.94}$ & $0.97$ & & $\boldsymbol{51.76}$  & $15.61$ \\

\bottomrule
\end{tabular}}
\label{tab:wiener_mse_ssim_results}
\end{table*}

% Tab 5.2: mIoU Results on ICNet (L_infty) 
% Table for mIoU comparison on the Cityscapes validation set with ICNet.
\begin{table*}[t!]
\centering
\caption{\textbf{Comparison of mIoU (in \%)} with and without denoising for the ICNet~\cite{Zhao2018a} model trained on the Cityscapes dataset. We report the mIoU w.r.t. the reference clean images $\boldsymbol{x}$ of (a) the \textbf{attacked} images $\boldsymbol{x}^{\text{adv}}$, (b) the \textbf{attacked denoised} images $\hat{\boldsymbol{x}}$, and (c) the \textbf{clean filtered} images $\boldsymbol{x}'$ over the entire \textbf{validation set} $\mathcal{D}_{\text{CS}}^{\text{val}}$ with adversarial examples ($\epsilon=10$ based on $\boldsymbol{L_{\infty}}$ norm). In the case of Wiener filtering, the filters are computed over clean and adversarial images with strength $\epsilon=5$ (\textbf{unmatched} conditions) and $\epsilon=10$ (\textbf{matched} conditions) spanning the entire training set. Best results are shown in \textbf{bold}, second best \underline{underlined} with the Wiener filter upper limit being excluded. The values in Fig. 5(c) are taken from the right-most column of this table.}
\label{tab:mIoU_results_ICNet}

\resizebox{\linewidth}{!}{
\begin{tabular}{c|c|cc|c|c|c|c|c|c|c|c} 
\toprule

\multicolumn{2}{c}{} & \multirow{2}{*}{\textbf{Defense Method / Attack Type}} &    & \textbf{none} & \textbf{mFGSM}  & \textbf{mFGSM}  & \textbf{Metzen}  & \textbf{Metzen}  &  \textbf{I.M.}  & \textbf{Mopuri} &  \textbf{All attacks} \\ 
 
  \multicolumn{4}{c|}{} & (\textbf{clean}) & \textbf{(Car)} & \textbf{(Ped)} & \textbf{(Car)} & \textbf{(Ped)}
&  &  & \textbf{(mean)} \\ 
 \hline

\multicolumn{4}{c|}{Baseline mIoU (\%)} & $67.25$ & $20.23$ & $20.39$ & $64.61$ & $65.73$ & $42.87$ & $27.65$ & $40.24$ \\ \hline

   \multirow{14}{*}{\rotatebox{90}{mIoU (\%) Denoised}} & \multirow{9}{*}{\rotatebox{90}{Wiener (Ours)}} & \multicolumn{2}{c|}{$\boldsymbol{G}$ (upper limit)}  & $67.25$ & $35.97$ & $36.53$ & $65.77$ & $66.49$ & $50.31$ & $41.27$ & $49.39$ \\ \cline{3-12}
   
   &   & \multirow{2}{*}{$\boldsymbol{G}^{(a)}$} & matched   & $66.43$ & \underline{$32.53$} & $33.05$ & $65.48$ & $66.22$ & $46.60$ & \underline{$38.96$} & $47.14$ \\
   
   &   &  & unmatched & $67.03$ & $28.37$ & $28.73$ & $65.14$ & $66.03$ & $44.67$ & $33.75$ & $44.45$ \\ \cline{3-12}

      &   & \multirow{2}{*}{$\boldsymbol{G}^{(\text{Metzen})}$}  & matched  & $67.12$ & $24.98$ & $25.14$ & $65.47$ & $66.22$ & $46.29$ & $31.20$ & $43.22$ \\
      
      &   &  & unmatched & \underline{$67.18$} & $22.75$ & $22.91$ & $65.13$ & $66.03$ & $44.44$ & $29.54$ & $41.80$ \\\cline{3-12}
      
      &   & \multirow{2}{*}{$\boldsymbol{G}^{(\text{mFGSM})}$}  & matched  & $65.54$ & \underline{$32.53$} & \underline{$33.18$} & $66.07$ & $66.07$ & $53.75$ & $37.37$ & $48.16$ \\
      
       &   &  & unmatched & $66.85$ & $28.37$ & $28.75$ & $65.84$ & $66.39$ & $49.41$ & $34.16$ & $45.49$ \\ \cline{3-12}
       
        &   & \multirow{2}{*}{$\boldsymbol{G}^{(\mathcal{A})}$}  & matched & $66.76$ & $28.82$ & $29.14$ & $65.94$ & $66.38$ & $49.98$ & $35.02$ & $45.88$ \\
    
     &   &  & unmatched & $67.07$ & $25.43$ & $25.60$ & $65.51$ & $66.26$ & $46.70$ & $31.80$ & $43.55$ \\
       \cline{2-12}
       
       & \multicolumn{3}{c|}{JPEG Compression} & $66.99$ & $20.27$ & $20.05$ & $65.03$ & $65.80$ & $46.72$ & $27.94$ & $40.96$ \\
       
  & \multicolumn{3}{c|}{JPEG 2000 compression} & $\boldsymbol{67.25}$ & $20.12$ & $20.25$ & $64.61$ & $65.73$ & $42.87$ & $27.52$ & $40.18$ \\
  
  & \multicolumn{3}{c|}{NL Means} & $65.50$ & $27.20$ & $27.49$ & $66.45$ & $66.48$ & $55.20$ & $33.44$ & $46.04$ \\
  
  & \multicolumn{3}{c|}{Median Blur} & $67.05$ & $21.59$ & $20.98$ & $65.64$ & $66.47$ & $47.64$ & $28.41$ & $41.78$ \\
  
  & \multicolumn{3}{c|}{Bit Depth Reduction} & $62.07$ & $19.77$ & $19.77$ & $62.24$ & $62.88$ & $45.87$ & $26.80$ & $39.55$ \\ \cline{2-12}
  
  & \multicolumn{3}{c|}{WF $\boldsymbol{G}^{(\mathcal{A})}$ (matched) + NL Means} & $65.18$ & $\boldsymbol{35.87}$ & $\boldsymbol{37.07}$ & \underline{$66.46$} & \underline{$66.49$} & $\boldsymbol{59.65}$ & $\boldsymbol{41.65}$ & $\boldsymbol{51.19}$ \\
       
    & \multicolumn{3}{c|}{WF $\boldsymbol{G}^{(\mathcal{A})}$ (unmatched) + NL Means} & $65.47$ & $32.22$ & $32.93$ & $\boldsymbol{66.83}$ & $\boldsymbol{66.93}$ & \underline{$57.95$} & $38.44$ & \underline{$49.21$} \\
 
\bottomrule
 
\end{tabular}}
\label{tab:wiener_mIoU_results_ICNet}
\end{table*}

% Tab 5.5: mIoU Results on FCN (L_infty)
% Table for mIoU comparison on the Cityscapes validation set with FCN.
\begin{table*}[t!]
\centering
\caption{\textbf{Comparison of mIoU (in \%)} with and without denoising for the FCN model trained on the Cityscapes dataset. We report the mIoU w.r.t. the reference clean images $\boldsymbol{x}$ of (a) the \textbf{attacked} images $\boldsymbol{x}^{\text{adv}}$, (b) the \textbf{attacked denoised} images $\hat{\boldsymbol{x}}$, and (c) the \textbf{clean filtered} images $\boldsymbol{x}'$ over the entire \textbf{validation set} with adversarial examples ($\epsilon=10$ for mFGSM and Mopuri; and $\epsilon=40$ for Iterative Mirror and Metzen attacks, both based on $\boldsymbol{L}_{\infty}$ norm). In the case of Wiener filtering, the filters are computed over clean and adversarial images with strength $\epsilon=10, 40$ (\textbf{matched} conditions) spanning the entire training set  $\mathcal{D}^{\text{train}}_{\text{DS}}$. Best results are shown in \textbf{bold}, second best \underline{underlined} with the Wiener filter upper limit being excluded. The values in Fig. 5(c) of the paper are taken from the right-most column of this table.}
\label{tab:mIoU_results_FCN}

\resizebox{0.9\linewidth}{!}{
\begin{tabular}{c|c|c|c|c|c|c|c|c|c|c} 
\toprule

\multicolumn{2}{c}{} & \multirow{2}{*}{\textbf{Defense Method / Attack Type}} &  \textbf{none} & \textbf{mFGSM}  & \textbf{mFGSM}  & \textbf{Metzen}  & \textbf{Metzen}  &  \textbf{I.M.}  & \textbf{Mopuri} &  \textbf{All attacks} \\ 
 
  \multicolumn{3}{c|}{} & (\textbf{clean}) & \textbf{(Car)} & \textbf{(Ped)} & \textbf{(Car)} & \textbf{(Ped)}
&  &  & \textbf{(mean)} \\ 
 \hline

\multicolumn{3}{c|}{Baseline mIoU (\%)} & $48.48$ & $20.97$ & $20.65$ & $28.30$  & $31.39$  & $19.77$ & $30.42$ & $28.56$ \\ \hline

   \multirow{11}{*}{\rotatebox{90}{mIoU (\%) Denoised}} & \multirow{5}{*}{\rotatebox{90}{WF (ours)}} & $\boldsymbol{G}$ (upper limit)  & $48.48$  & $29.84$  & $29.86$ & $36.75$  &  $38.92$ & $31.42$ & $37.81$ & $36.15$ \\ \cline{3-11}
   
   &   & $\boldsymbol{G}^{(a)}$ & $48.15$  & $\underline{27.93}$ & $\underline{27.60}$  & $\underline{34.99}$ & $37.33$ & $\underline{27.89}$ & $\underline{37.28}$ & $\underline{32.17}$ \\ \cline{3-11}

      &   & $\boldsymbol{G}^{(\text{Metzen\_Car})}$ & $48.28$ & $27.25$ & $26.95$ & $\underline{34.99}$ & $37.33$ & $27.60$ & $34.92$ & $31.50$ \\ \cline{3-11}

      &   & $\boldsymbol{G}^{(\text{mFGSM})}$ & $48.12$ & $\underline{27.93}$  &  $\underline{27.60}$  & $34.95$ &  $\underline{37.38}$ & $27.84$ & $35.85$ & $31.92$ \\ \cline{3-11}

        &   & $\boldsymbol{G}^{(\mathcal{A})}$ & $48.21$ & $27.52$ & $27.38$  & $\underline{34.99}$ & $37.26$ & $27.56$ & $35.87$ & $31.76$ \\  \cline{2-11}

  & \multicolumn{2}{c|}{JPEG Compression} & $48.09$  & $23.30$ & $23.06$ & $30.98$ & $34.18$ & $23.04$ & $31.64$ & $27.70$ \\
       
  & \multicolumn{2}{c|}{JPEG 2000 compression} & $\boldsymbol{48.48}$  & $23.06$  &  $22.99$ & $30.57$  & $33.84$ & $22.19$  & $31.89$ & $27.41$ \\
  
  & \multicolumn{2}{c|}{NL Means} & $48.03$ & $24.62$ &  $24.64$ & $32.44$ & $35.67$ & $24.47$ & $33.26$ & $29.17$ \\
  
  & \multicolumn{2}{c|}{Median Blur} & $\underline{48.42}$ & $23.46$ & $23.49$ & $31.66$ & $34.92$ & $23.52$ &  $32.11$ & $28.19$ \\
  
  & \multicolumn{2}{c|}{Bit Depth Reduction} &  $46.39$ & $22.86$ & $22.76$ & $30.82$ & $33.99$ & $22.63$ & $31.27$ & $27.38$ \\ \cline{2-11}
  
  & \multicolumn{2}{c|}{WF $\boldsymbol{G}^{(\mathcal{A})}$ + NL Means} & $47.78$ & $\boldsymbol{29.60}$ & $\boldsymbol{29.33}$ & $\boldsymbol{37.36}$ & $\textbf{39.12}$  & $\boldsymbol{30.59}$ & $37.08$ & $\boldsymbol{33.84}$ \\
       
\bottomrule
 
\end{tabular}}
\label{tab:wiener_mIoU_results_FCN}
\end{table*}
